# Supplementary material for: CrowdMoGen: Zero-Shot Text-Driven Collective Motion Generation
Source: arXiv:2407.06188 source file (2025-05-09)
Supplement: Supplementary file 1 [file 7_supp.tex]

\appendix

% \tableofcontents
% \clearpage

\section{Details of CrowdMoGen}

\subsection{Diffusion Model}
\label{sec:diffusion}

Diffusion models can be defined using a Markov chain $p_{\theta}(\mathbf{x}_0)\,:=\,\int{p_{\theta}(\mathbf{x}_{0:T})\,d{\mathbf{x}_{1:T}}}$, where the intermediate variables $\mathbf{x}_{1},\cdots,\mathbf{x}_{T}$ represent noised versions of the original data $\mathbf{x}_0 \sim q(\mathbf{x}_0)$, and maintains the same dimensionality as the original data. In motion generation, every $\mathbf{x}_t$ corresponds to a motion sequence $\theta_i \in \mathbb{R}^D, i=1,2,\dots,F$, where $D$ denotes the dimensionality of each pose, and $F$ represents the total number of frames. In the diffusion process of diffusion models, ~\cite{ho2020denoising} efficiently derive $\mathbf{x}_t$ from $x_0$ by approximating $q(\mathbf{x}_t)$ as $\mathbf{x}:=\sqrt{\bar{\alpha}_t} \mathbf{x}_0 + \sqrt{1 - \bar{\alpha}_t}\epsilon$, where $\alpha_t := 1 - \beta_t$, $\bar{\alpha}_t:=\prod_{s=1}^t \alpha_s$, and $\beta_t$ is a predefined variance schedule at the $t^{\text{th}}$ noising step. 
Then, the diffusion process is reversed for clean motion recovery. Specifically, a motion generation model $S$ is configured to refine noisy data $\mathbf{x}_t$ back to its original, clean state $\mathbf{x}_0$. Following approaches like MDM~\cite{tevet2022human} and ReMoDiffuse~\cite{zhang2023remodiffuse}, we estimate $\mathbf{x}_0$ as $S(\mathbf{x}_t,t,c)$, where $c$ represents the conditioning signal containing the spatial control signal $c^s$ and the textual control signal $c^t$, and $t \in \mathcal{U}(0, T)$ marks the timestep in the diffusion process. Finally in the sampling phase, we derive $\mathbf{x}_{t-1}$ by sampling it from the Gaussian distribution $\mathcal{N}(\mu_{\theta}(\mathbf{x}_t,t,c), \beta_t)$, where the mean is specified as follows:
\begin{equation}
    \begin{aligned}
    & \mu_{\theta}(\mathbf{x}_t,t,c) = \sqrt{\bar{\alpha}_t} S(\mathbf{x}_t,t,c) + \sqrt{1 - \bar{\alpha}_t}\epsilon_{\theta}(\mathbf{x}_t,t,c), \\
    & \epsilon_{\theta}(\mathbf{x}_t,t,c)=(\frac{\mathbf{x}_t}{\sqrt{\bar{\alpha}_t}} - S(\mathbf{x}_t,t,c)) \sqrt{\frac{1}{\bar{\alpha}_t}-1}.
    \end{aligned}
\end{equation}

\subsection{Human Motion Representation. } 

Human motion can be parameterized using two primary methods: relative or global joint representation. The relative representation, proposed in ~\cite{guo2022generating}, is a redundant format that includes pelvis velocity, local joint positions, velocities, and rotations relative to the pelvis, complemented by foot contact binary labels. This method simplifies the model learning process and supports the generation of natural human motions aligning with inherent human body priors. However, it faces challenges in precise spatial control, especially in sparse time frames and when controlling joints beyond the pelvis, due to its lack of a stable global reference. Consequently, controlling methods~\cite{tevet2022human, karunratanakul2023guided} using this format struggle with consistency and precision in joint-wise spatial control across timesteps.
% global
In contrast, global joint representation provides each joint’s absolute coordinates within a global framework, offering clear and direct reference for fine-grained control. Therefore, inspired by~\cite{xie2023omnicontrol}, we employ a hybrid approach to represent motions in our framework: utilizing relative representation for training and routine generation, and switching to global positioning for enhanced spatial control.

\subsection{IK Guidance}

Noise optimization during the sampling stage enhances the spatial control capabilities of our model. In each diffusion step, gradient descent optimization is performed on the output mean in response to the input spatial control signals. Specifically, $\mathcal{D}(\mu_{\theta}(\mathbf{x}_t,t,c), c^s)$ quantifies the discrepancy between the currently generated mean $\mu_{\theta}(\mathbf{x}_t,t,c)$ and the provided spatial signal $c^s$. To ensure precise control, we selectively supervise specific time frames and joints, while masking unsupervised components. 
\begin{equation}
    \begin{aligned}
    \mathcal{D}(\mu_{\theta}(\mathbf{x}_t,t,c), c_s) = \frac{\sum_{i} \sum_{j} O_{ij} \| c_{ij}^{s} - \mu^{g}_{ij} \|_{2}}{\sum_{i} \sum_{j} O_{ij}}
    \end{aligned}
\end{equation}
Here, $O_{ij}$ is a boolean value representing if at frame $i$, joint $j$ is controlled. The predicted mean is transformed into a global joint representation $\mu^g$ and assessed with the control signal $c^s$ in the same format, ensuring that joint positions align with the spatial control requirements from a global perspective in both time and layout. Additionally, since gradient updates target the mean $\mathbf{x}_t$ in a relative motion representation, these updates are naturally propagated across all time frames and joints throughout the motion sequence. This coherent propagation facilitates a natural adjustment of the entire body’s joints, even when only a few joints are being actively controlled and edited.

\section{Details of Experiments}
% \begin{wrapfigure}{r}{0.45\textwidth}
%   \centering
%   \includegraphics[width=\linewidth, keepaspectratio]{images/user_study_instruction.png}
%   \caption{\textbf{Example of the evaluation instructions of the user study.}}
%   \label{fig:userstudyins}
%   % \vspace{-30px}
% \end{wrapfigure}
% \begin{wrapfigure}{r}{0.45\textwidth}
%   \centering
%   \includegraphics[width=\linewidth, keepaspectratio]{images/user_study_question.png}
%   \caption{\textbf{Example of the questions of the user study.}}
%   \label{fig:userstudyquestion}
%   % \vspace{-30px}
% \end{wrapfigure}

\begin{figure}[h]
  \centering
  \begin{minipage}{0.45\textwidth}
    \centering
    \includegraphics[width=\linewidth]{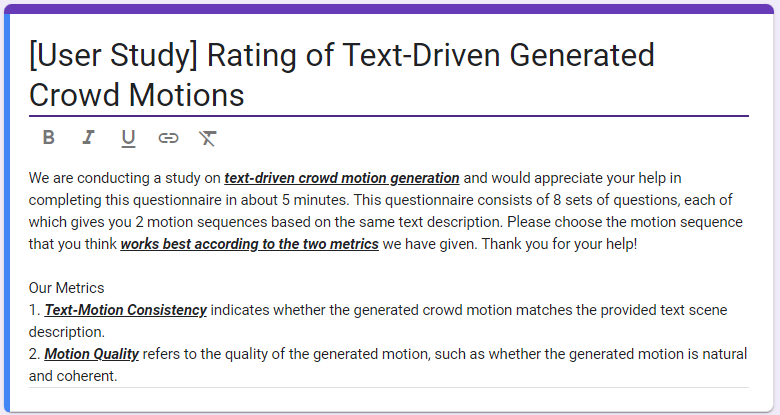} % first figure itself
    \caption{\textbf{Example of the evaluation instructions of the user study.}}
    \label{fig:userstudyins}
  \end{minipage}\hfill
  \begin{minipage}{0.45\textwidth}
    \centering
    \includegraphics[width=\linewidth]{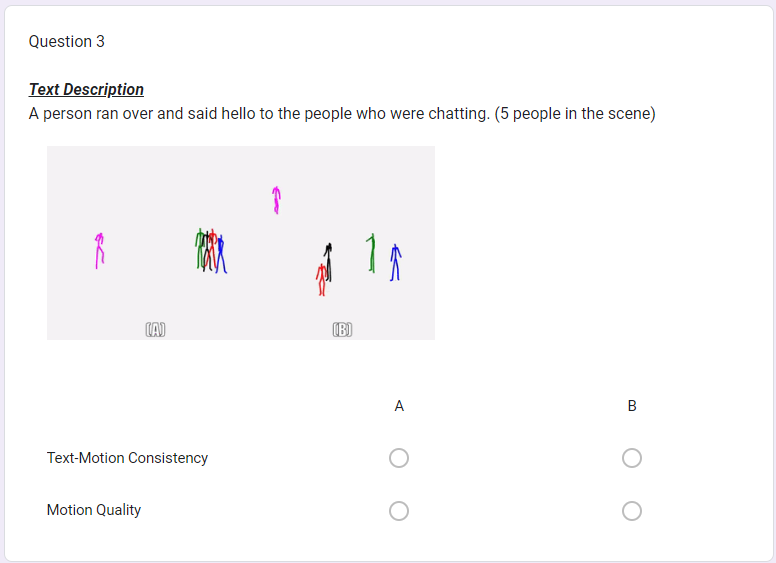} % second figure itself
    \caption{\textbf{Example of the questions of the user study.}}
    \label{fig:userstudyquestion}
  \end{minipage}
\end{figure}

\subsection{Details of User Study}
In our user study, we developed a questionnaire and generated 8 random scenarios using our proposed method. The evaluation instructions and a comparison example of these scenarios are illustrated in Figure~\ref{fig:userstudyins} and Figure~\ref{fig:userstudyquestion}. We recruited 50 participants aged between 20 and 35, comprising animators, AI researchers, and gaming enthusiasts, to partake in the study. Participants were presented with textual descriptions and asked to evaluate crowd motions planned by our module against those planned by the original GPT-4, focusing on the quality of the motion and its consistency with the text. Our findings indicate that the plain GPT-4, lacking specialized prompt engineering, often fails to seamlessly integrate joint interactions, global paths, and comprehensive motion planning. In contrast, our module utilizes a sophisticated tree-of-thought approach that strategically segments planning into macro and micro levels. 

\subsection{Details of Evaluation Metrics}
Detailed explanations of the metrics and the methods used are provided here due to article length constraints.
\par
\textbf{Semantic-Level Evaluation Metrics}
The following metrics are usually used to evaluate traditional text-to-motion task. To quantitatively assess, motion and text feature extractors are developed and trained under contrastive loss to produce feature vectors that are close geometrically for matching text-motion pairs and distant for non-corresponding pairs. \textbf{(1) R-Precision:} A pool is formed from the accurate description of a generated motion and 31 unrelated descriptions from the test dataset. Euclidean distances between the motion's features and those of each description in the pool are calculated and ranked. Accuracy is then averaged at the top-1, top-2, and top-3 levels, with successful retrievals marked by the ground truth description appearing within the top-k selections. \textbf{(2) MultiModality:} A distance is calculated by averaging the Euclidean distances between each generated motion's features and the text features of its respective description in the test set. \textbf{(3) Frechet Inception Distance (FID):} FID reflects the generation quality by calculating the distance between features extracted from real and generated motion sequences. \textbf{(4) Diversity:} Diversity measures the variability and richness of the generated motion sequences. \textbf{(5) Multi-Modality:} Multi-modality measures the average variance of different generated motion sequences given a single text description.
We use R-Precision, FID, and Diversity for evaluating our method on the text-to-motion task, since these metrics can best showcase the generation quality and control ability of a model.

\textbf{Spatial-Level Evaluation Metrics}: Metrics such as Foot skating ratio, Trajectory error, Location error, and Average error of keyframe locations are employed to evaluate our proposed method's spatial control ability.  \textbf{(1) Trajectory error} refers to the proportion of trajectories that are unsuccessful, which occurs when any keyframe's location error exceeds a set threshold. \textbf{(2) Average error} is computed as the mean distance between the positions of generated motions and the actual keyframe positions observed during the key motion steps. \textbf{(3) Location error} represents the ratio of keyframe locations that are not fall within a threshold distance.  \textbf{(3) Foot skating ratio} is a metric used to quantify the amount of sliding or unrealistic movements of feet in animations.
\section{Dataset License}

\subsection{AMASS License}

Dataset Copyright License for non-commercial scientific research purposes
Please read carefully the following terms and conditions and any accompanying documentation before you download and/or use the AMASS Dataset and the accompanying Software (jointly refered to as the "Dataset"). By downloading and/or using the Dataset, you acknowledge that you have read these terms and conditions, understand them, and agree to be bound by them. If you do not agree with these terms and conditions, you must not download and/or use the Dataset. Any infringement of the terms of this agreement will automatically terminate your rights under this License

Ownership / Licensees
The Dataset and the associated materials has been developed at the Max Planck Institute for Intelligent Systems (hereinafter "MPI"). Any copyright or patent right is owned by and proprietary material of the Max-Planck-Gesellschaft zur Förderung der Wissenschaften e.V. (hereinafter “MPG”; MPI and MPG hereinafter collectively “Max-Planck”) hereinafter the “Licensor”.

License Grant
Licensor grants you (Licensee) personally a single-user, non-exclusive, non-transferable, free of charge right:

To obtain and install the Dataset on computers owned, leased or otherwise controlled by you and/or your organization;
To use the Dataset for the sole purpose of performing non-commercial scientific research, non-commercial education, or non-commercial artistic projects;
Any other use, in particular any use for commercial purposes, is prohibited. This includes, without limitation, incorporation in a commercial product, use in a commercial service, or production of other artefacts for commercial purposes. The Dataset may not be reproduced, modified and/or made available in any form to any third party without Max-Planck’s prior written permission. 

The Dataset may not be used for pornographic purposes or to generate pornographic material whether commercial or not. This license also prohibits the use of the Dataset to train methods/algorithms/neural networks/etc. for commercial use of any kind. By downloading the Dataset, you agree not to reverse engineer it.

No Distribution
The Dataset and the license herein granted shall not be copied, shared, distributed, re-sold, offered for re-sale, transferred or sub-licensed in whole or in part except that you may make one copy for archive purposes only.

Disclaimer of Representations and Warranties
You expressly acknowledge and agree that the Dataset results from basic research, is provided “AS IS”, may contain errors, and that any use of the Dataset is at your sole risk. LICENSOR MAKES NO REPRESENTATIONS OR WARRANTIES OF ANY KIND CONCERNING THE SOFTWARE, NEITHER EXPRESS NOR IMPLIED, AND THE ABSENCE OF ANY LEGAL OR ACTUAL DEFECTS, WHETHER DISCOVERABLE OR NOT. Specifically, and not to limit the foregoing, licensor makes no representations or warranties (i) regarding the merchantability or fitness for a particular purpose of the Dataset, (ii) that the use of the Dataset will not infringe any patents, copyrights or other intellectual property rights of a third party, and (iii) that the use of the Dataset will not cause any damage of any kind to you or a third party.

Limitation of Liability
Because this Software License Agreement qualifies as a donation, according to Section 521 of the German Civil Code (Bürgerliches Gesetzbuch – BGB) Licensor as a donor is liable for intent and gross negligence only. If the Licensor fraudulently conceals a legal or material defect, they are obliged to compensate the Licensee for the resulting damage.
Licensor shall be liable for loss of data only up to the amount of typical recovery costs which would have arisen had proper and regular data backup measures been taken. For the avoidance of doubt Licensor shall be liable in accordance with the German Product Liability Act in the event of product liability. The foregoing applies also to Licensor’s legal representatives or assistants in performance. Any further liability shall be excluded.
Patent claims generated through the usage of the Dataset cannot be directed towards the copyright holders.
The contractor points out that add-ons as well as minor modifications to the Dataset may lead to unforeseeable and considerable disruptions.

No Maintenance Services
You understand and agree that Licensor is under no obligation to provide either maintenance services, update services, notices of latent defects, or corrections of defects with regard to the Dataset. Licensor nevertheless reserves the right to update, modify, or discontinue the Dataset at any time.

Defects of the Dataset must be notified in writing to the Licensor with a comprehensible description of the error symptoms. The notification of the defect should enable the reproduction of the error. The Licensee is encouraged to communicate any use, results, modification or publication.

\subsection{HumanML3D License}

MIT License

Copyright (c) 2022 Chuan Guo

Permission is hereby granted, free of charge, to any person obtaining a copy
of this software and associated documentation files (the "Software"), to deal
in the Software without restriction, including without limitation the rights
to use, copy, modify, merge, publish, distribute, sublicense, and/or sell
copies of the Software, and to permit persons to whom the Software is
furnished to do so, subject to the following conditions:

The above copyright notice and this permission notice shall be included in all
copies or substantial portions of the Software.

THE SOFTWARE IS PROVIDED "AS IS", WITHOUT WARRANTY OF ANY KIND, EXPRESS OR
IMPLIED, INCLUDING BUT NOT LIMITED TO THE WARRANTIES OF MERCHANTABILITY,
FITNESS FOR A PARTICULAR PURPOSE AND NONINFRINGEMENT. IN NO EVENT SHALL THE
AUTHORS OR COPYRIGHT HOLDERS BE LIABLE FOR ANY CLAIM, DAMAGES OR OTHER
LIABILITY, WHETHER IN AN ACTION OF CONTRACT, TORT OR OTHERWISE, ARISING FROM,
OUT OF OR IN CONNECTION WITH THE SOFTWARE OR THE USE OR OTHER DEALINGS IN THE
SOFTWARE.

\subsection{KIT-ML License}

The MIT License (MIT)

Copyright (c) 2016 Matthias Plappert

Permission is hereby granted, free of charge, to any person obtaining a copy
of this software and associated documentation files (the "Software"), to deal
in the Software without restriction, including without limitation the rights
to use, copy, modify, merge, publish, distribute, sublicense, and/or sell
copies of the Software, and to permit persons to whom the Software is
furnished to do so, subject to the following conditions:

The above copyright notice and this permission notice shall be included in all
copies or substantial portions of the Software.

THE SOFTWARE IS PROVIDED "AS IS", WITHOUT WARRANTY OF ANY KIND, EXPRESS OR
IMPLIED, INCLUDING BUT NOT LIMITED TO THE WARRANTIES OF MERCHANTABILITY,
FITNESS FOR A PARTICULAR PURPOSE AND NONINFRINGEMENT. IN NO EVENT SHALL THE
AUTHORS OR COPYRIGHT HOLDERS BE LIABLE FOR ANY CLAIM, DAMAGES OR OTHER
LIABILITY, WHETHER IN AN ACTION OF CONTRACT, TORT OR OTHERWISE, ARISING FROM,
OUT OF OR IN CONNECTION WITH THE SOFTWARE OR THE USE OR OTHER DEALINGS IN THE
SOFTWARE.
